# Supplementary material for: The Stochastic Parrot on LLM's Shoulder: A Summative Assessment of Physical Concept Understanding
Source: arXiv:2502.08946 source file (2025-02-13)
Supplement: Supplementary file 1 [file appendix.tex]

\section{More Details on Experiment Setup}
